# Supplementary material for: A Survey of the Usages of Deep Learning in Natural Language Processing
Source: arXiv:1807.10854 source file (2019-12-21)
Supplement: Supplementary file 1 [file supplement.tex]

\begin{figure*}%[t!]

    \centering
    
    \subfloat(a)
    %\begin{subfigure}{0.35\textwidth}
        %\centering
        \includegraphics[height=1.625in]{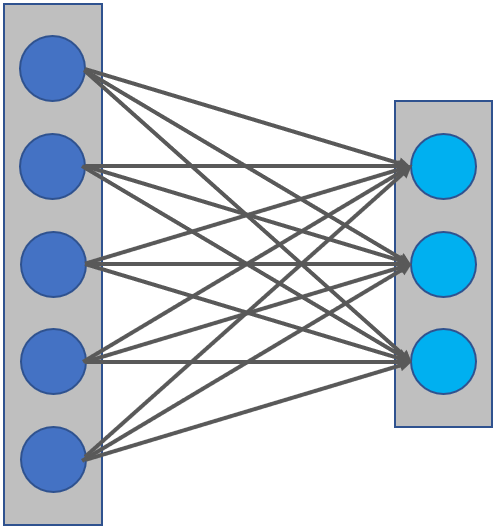}
        %\caption{Fully-Connected ANN}
        \label{figure:dense_ANN}
    %\end{subfigure}
    \hfil
    \subfloat(b)
    %\begin{subfigure}{0.25\textwidth}
        %\centering
        \includegraphics[height=1.625in]{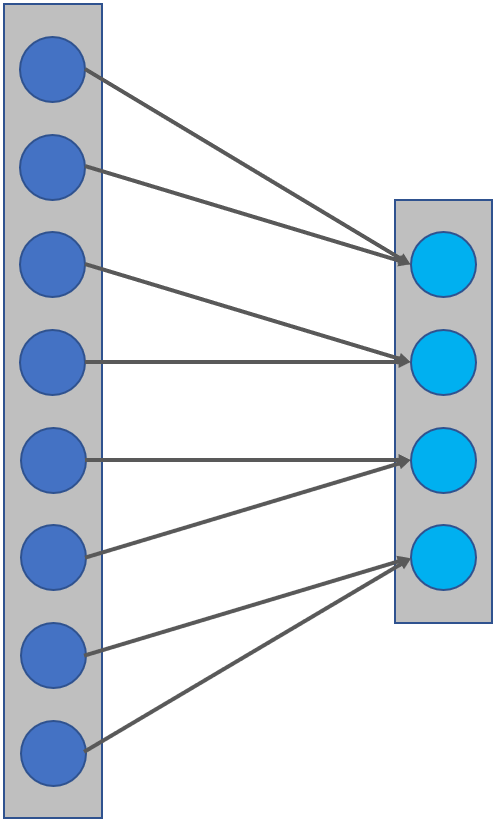}
        %\caption{Non-dense ANN}
        \label{figure:basic_ANN}
    %\end{subfigure}
    \hfil
    \subfloat(c)
    %\begin{subfigure}{0.4\textwidth}
        %\centering
        \includegraphics[height=1.625in]{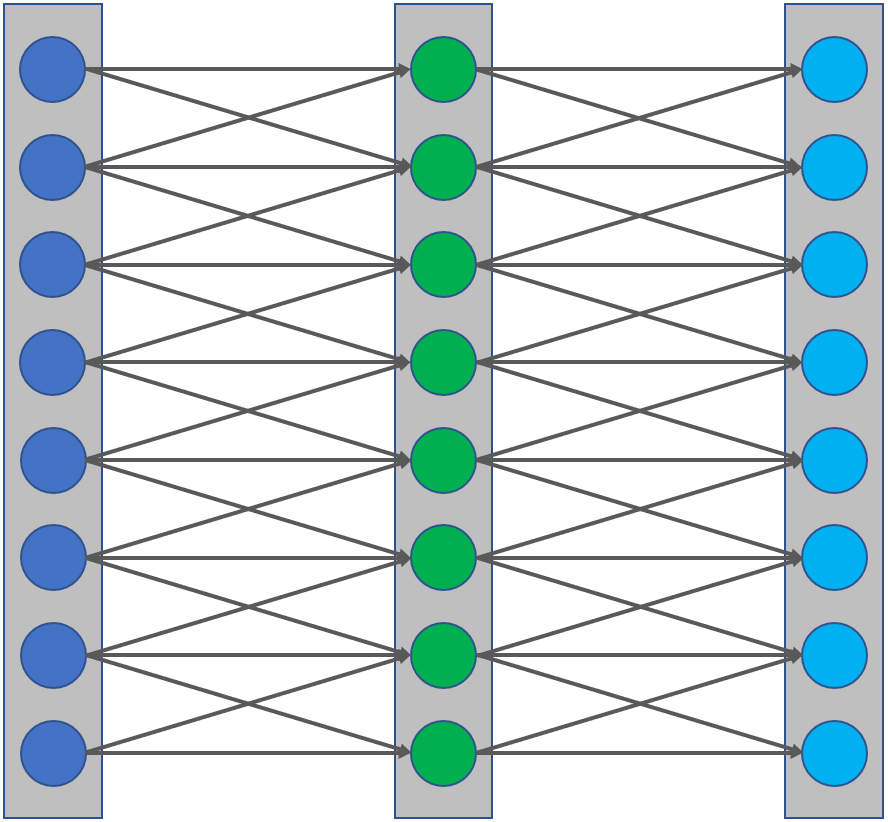}
        %\caption{ANN with Hidden Layer}
        \label{figure:ANN_with_hidden_layer}
    %\end{subfigure}

    \caption{Simple Neural Networks. Networks built until recently had very few layers. Early networks were fully connected as shown in (a), although non-dense networks, such as that shown in (b) are common these days. Layers that are neither the input nor output layers, as exhibited in (c), are said to be "hidden".}
    
    \label{figure:SimpleNetworks}
    
\end{figure*}
\begin{figure*}%[t!]

    \centering
    
    \subfloat(a)
    %\begin{subfigure}
        %\centering
        \includegraphics[height=1.625in]{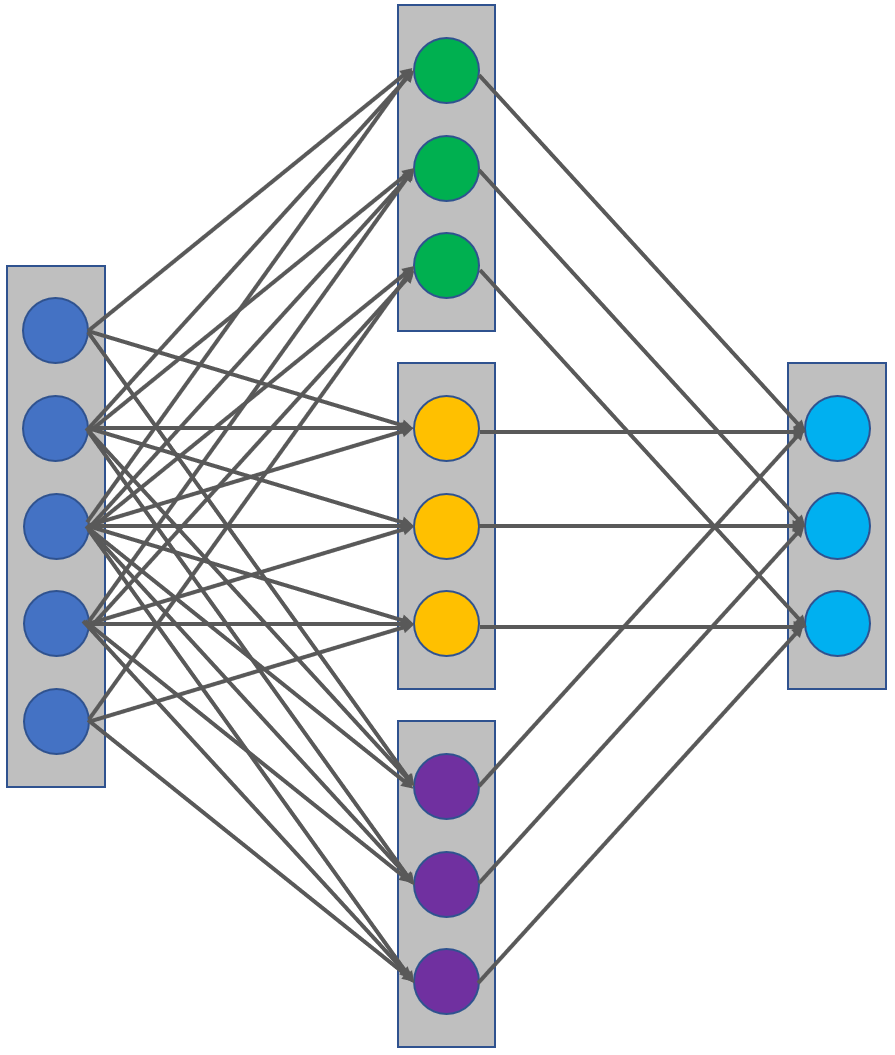}
        %\caption{Basic CNN}
        \label{figure:simple_CNN}
    %\end{subfigure}
    \hfil
    \subfloat(b)
    %\begin{subfigure}
        %\centering
        \includegraphics[height=1.625in]{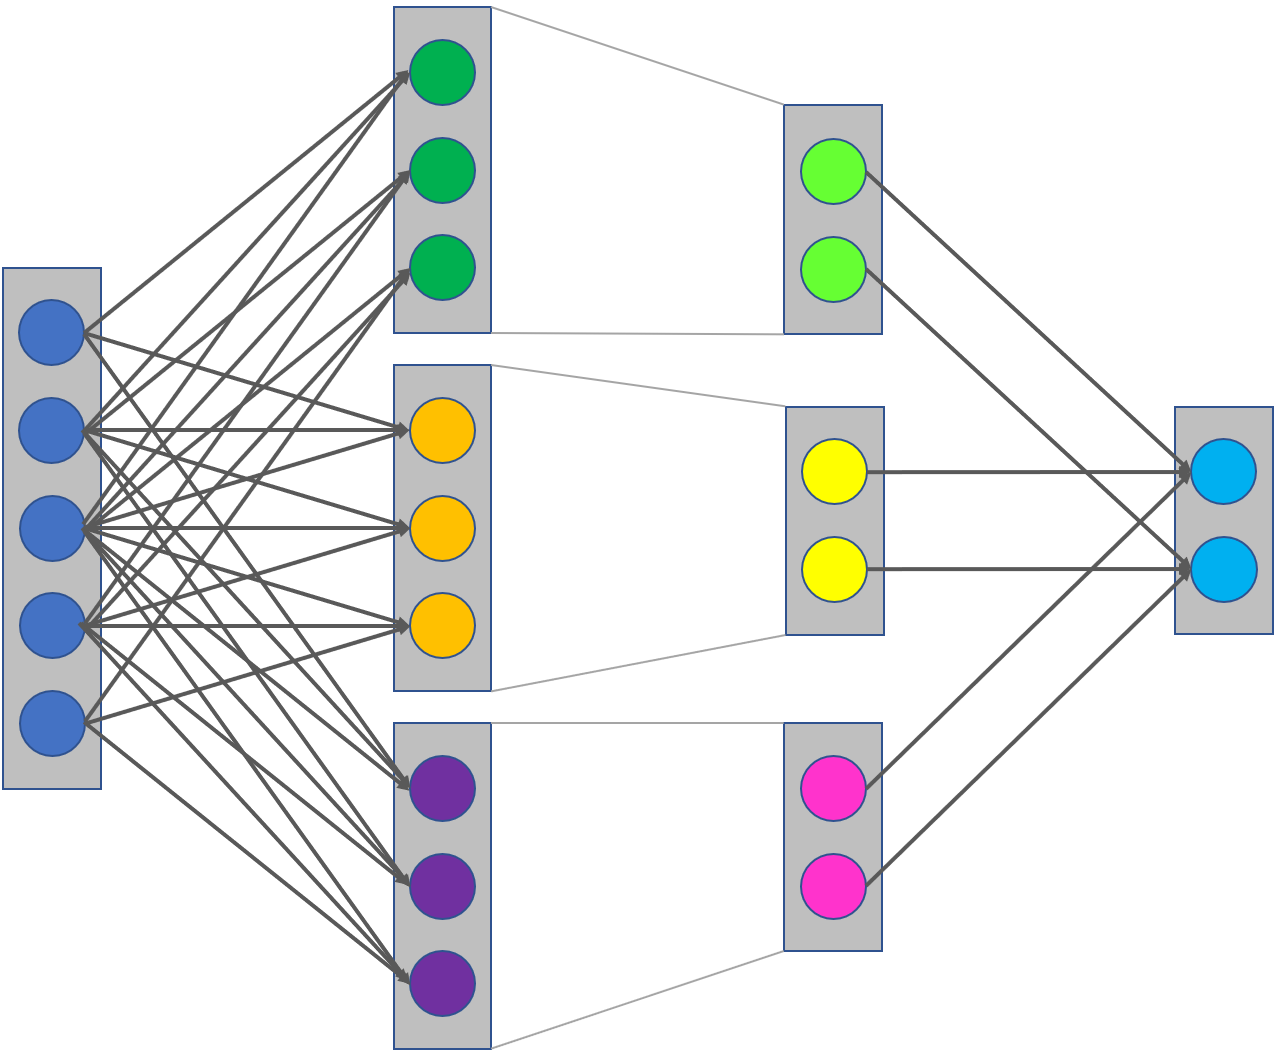}
        %\caption{CNN with Pooling}
        \label{figure:CNN_with_pooling}
    %\end{subfigure}
    
    \caption{Convolutional Neural Networks. These networks have three distinct filters that operate on the input layer, each with a receptive field size of three. In (b), $k$-max pooling is exhibited, where $k = 2$ with a pool size of three.}
    
    \label{figure:CNNs}
    
\end{figure*}

%\begin{figure}[!t]
%\centering
%\includegraphics[width=2.5in]{myfigure}
%\caption{Simulation results for the network.}
%\label{fig_sim}
%\end{figure}
\begin{figure*}[t!]

    \centering
    
    \subfloat(a)
    %\begin{subfigure}{0.33\textwidth}
        \centering
        \includegraphics[width=1.75in]{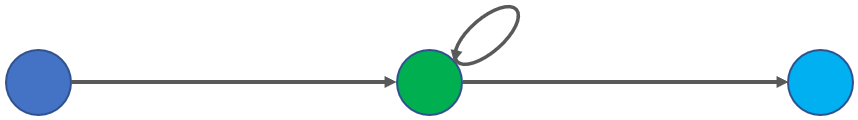}
        %\caption{Basic RNN}
        \label{figure:basic_RNN}
    %\end{subfigure}
    \hfil
    \subfloat(b)
    %\begin{subfigure}{0.67\textwidth}
        \centering
        \includegraphics[width=3.5in]{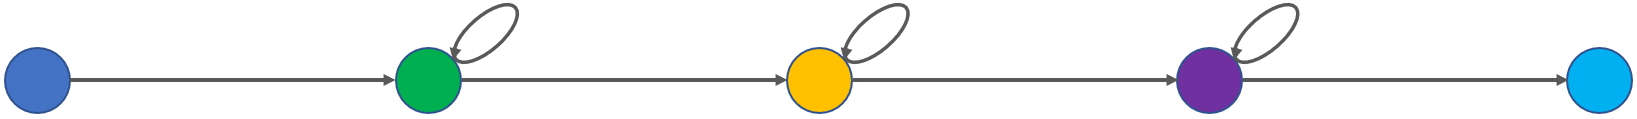}
        %\caption{Stacked RNN}
        \label{figure:stacked_RNN}
    %\end{subfigure}
    \vfil
    \subfloat(c)
    %\begin{subfigure}{0.33\textwidth}
        \centering
        \includegraphics[height=1in]{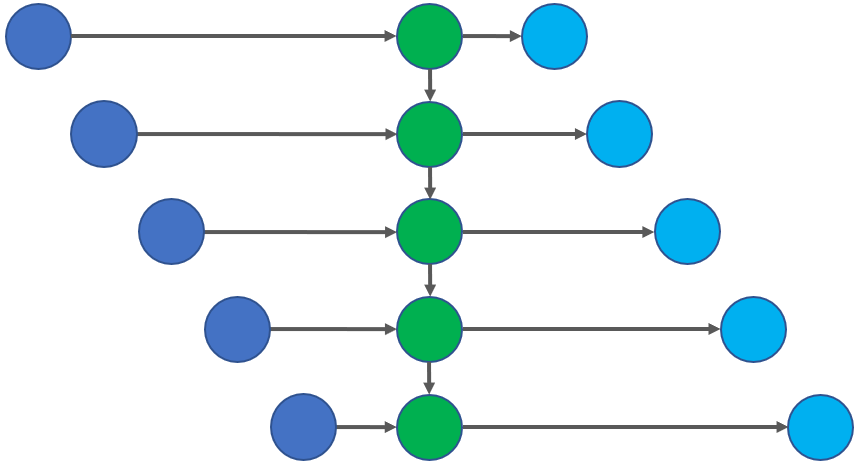}
        %\caption{Unrolled RNN}
        \label{figure:unrolled_RNN}
    %\end{subfigure}
    \hfil
    \subfloat(d)
    %\begin{subfigure}{0.33\textwidth}
        \centering
        \includegraphics[height=1in]{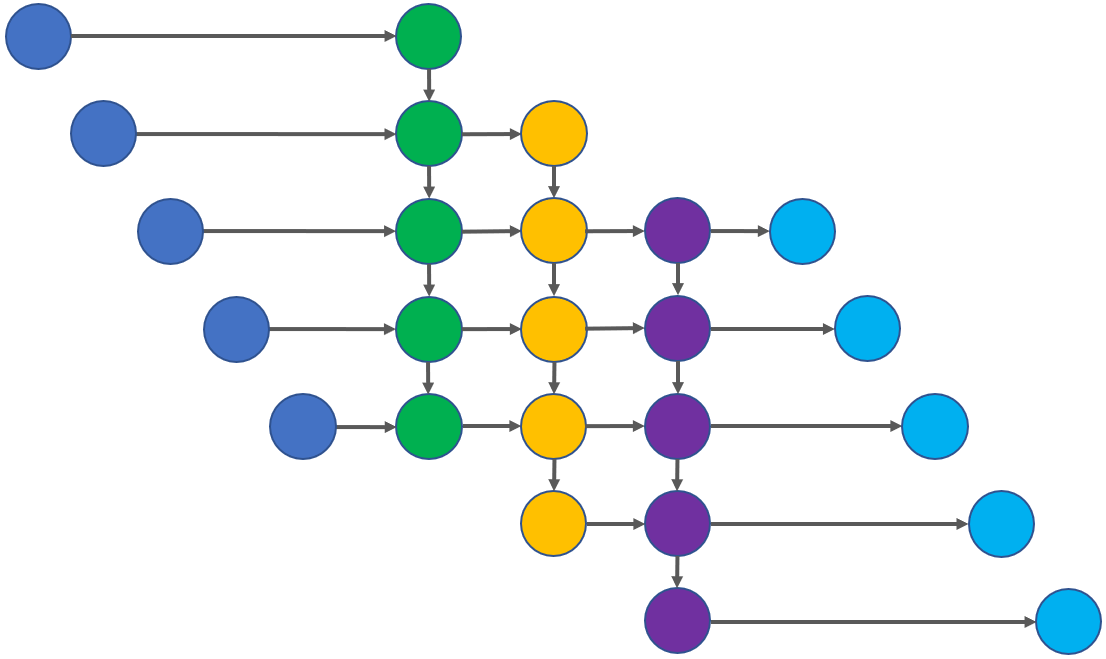}
        %\caption{Unrolled RNN Stack}
        \label{figure:stacked_RNN_unrolled}
    %\end{subfigure}
    \hfil
    \subfloat(e)
    %\begin{subfigure}{0.33\textwidth}
        \centering
        \includegraphics[height=1in]{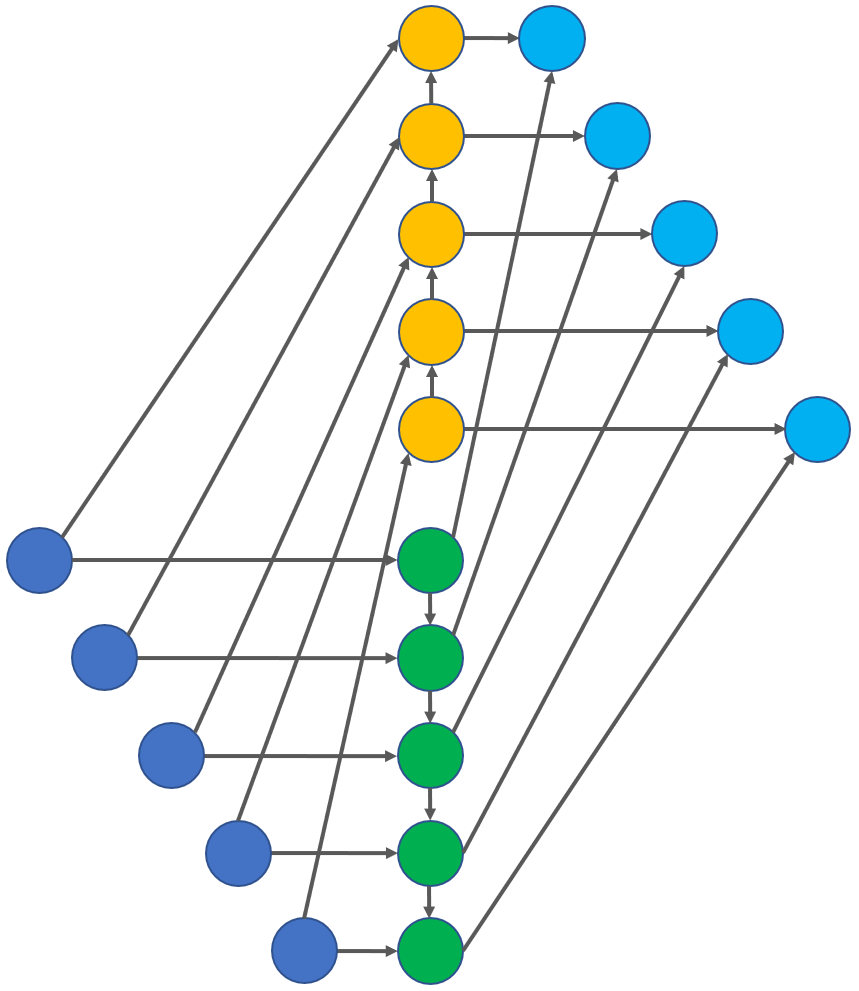}
        %\caption{Bidirectional RNN}
        \label{figure:bidirectional_RNN}
    %\end{subfigure}
    
    \caption{Recurrent Neural Networks. These networks can be "unrolled" to appear as multiple different nodes. Note that (a) and (c) are identical, as are (b) and (d). If an entire data sequence is known prior to computation beginning, RNNs can also operate over the reverse sequence of the data. Bidirectional networks such as (e) utilize two RNNs working in opposite directions and then combine the outputs.}
    
    \label{figure:RNNs}

\end{figure*}
\begin{figure}[h!]

    \centering
    
    \includegraphics[width=2.5in]{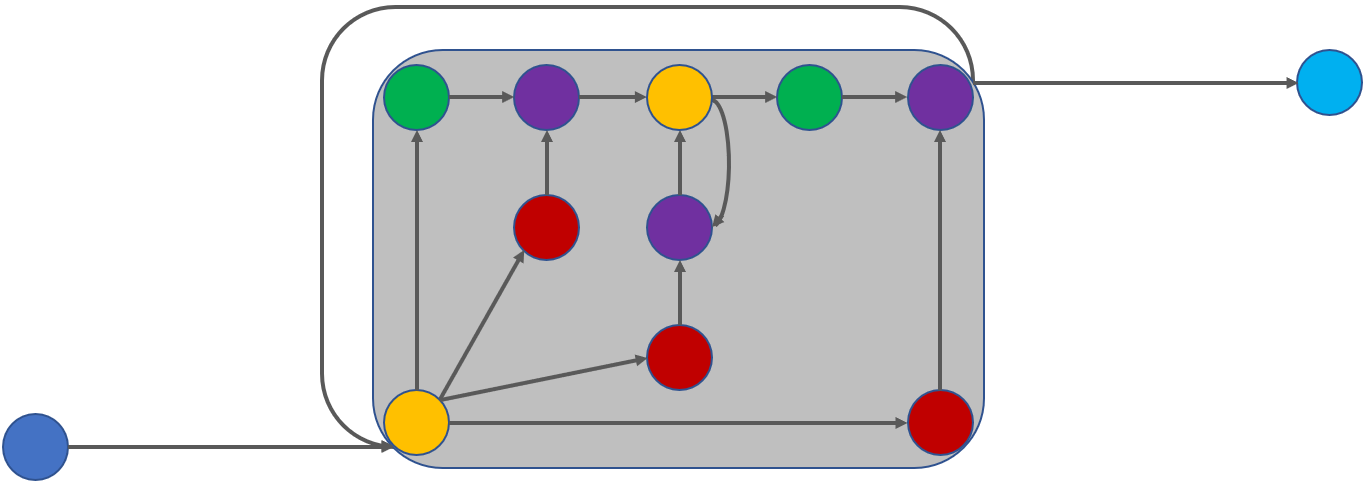}
    
    \caption{Long Short-Term Memory Network. In this network, the input is concatenated with the previous output and is then distributed to an activation node and to three sigmoid  nodes followed by gate nodes. Depending on the outputs of the sigmoid nodes, the gate nodes choose whether or not to allow information to pass through. These gates control i) the input, ii) the recurrent internal state, and iii) the output.}
    
    \label{figure:LSTM}

\end{figure}
